# Supplementary material for: Federated Koopman-Reservoir Learning for Large-Scale Multivariate Time-Series Anomaly Detection
Source: arXiv:2503.11255 source file (2025-03-14)
Supplement: Supplementary file 1 [file appendix2.tex]

\section{Additional Experiments}

\subsection{Other Federated Learning Baselines:}
\label{ap:additional_exp}

\begin{table*}[t]
\centering
\caption{Performance comparison across other FL approaches. Metrics with best performance are \underline{underline}.}
\label{tab:performance_fl}
 % For row height
\scalebox{0.87}{
\begin{tabular}{|c|c||c||c|c|c|c|c|c|c|c|}
\hline
\multirow{2}{*}{\textbf{Dataset}} & \multirow{2}{*}{\textbf{Metric}} & \multirow{2}{*}{\textbf{\textsc{FedKO}}} & \multicolumn{4}{c|}{\textbf{Scaffold}} & \multicolumn{4}{c|}{\textbf{FedProx}} \\ \cline{4-11} 
                &                &         & \textbf{\textsc{ReKo}}       & \textbf{USAD} & \textbf{GDN} & \textbf{TranAD} &  \textbf{\textsc{ReKo}} &  \textbf{USAD} & \textbf{GDN} & \textbf{TranAD} \\ 
                \hline
                \hline
\multirow{3}{*}{\textbf{PSM}}  & Pre  & \underline{\textbf{97.55}} & 97.15 & 90.61 & 94.81 & 79.17 & 96.51 & 96.78 & 96.52 & 70.44 \\
                      & Recall   & \underline{\textbf{89.89}} & 88.59 & 87.53 & 91.19 & 83.74 & 90.10 & 87.32 & 89.82 & 89.23 \\
                      & F1   & \underline{\textbf{93.56}} & 92.67 & 89.04 & 92.96 & 81.39 & 92.19 & 91.81 & 93.05 & 78.73 \\ \hline
\multirow{3}{*}{\textbf{SMD}}  & Pre  & \textbf{76.25} & 78.35 & 54.39 & 71.76 & 46.52 & 73.59 & 56.26 & \underline{90.23} & 48.23 \\
                      & Recall  & \textbf{79.75} & 75.53 &  71.28 & 60.72 & 35.05 & \underline{80.63} & 70.29 & 50.71 & 41.96 \\
                      & F1   & \underline{\textbf{77.95}} & 76.91 & 61.70 & 65.77 & 39.98 & 76.95 & 62.50 & 64.93 & 44.87 \\ \hline
\multirow{3}{*}{\textbf{SMAP}} & Pre  & \underline{\textbf{94.67}} & 93.72 & 92.37 & 94.63 & 91.66 & 92.47 & 92.39 & 87.15    & 87.56 \\
                      & Recall   & \textbf{57.25} & 56.49 & 54.92 & 54.92 & 55.04 & 57.01 & 54.92 & 60.39 & \underline{58.35} \\
                      & F1   & \underline{\textbf{71.35}} & 70.49 & 68.88 & 69.50 & 68.78 & 70.53 & 68.89 & 71.34 & 70.03 \\ \hline
\multirow{3}{*}{\textbf{MSL}}  & Pre  & \textbf{83.61} & 83.28 & 64.13 & 75.12 & 76.98 & 82.40 & 64.16 & 81.51 & \underline{89.29} \\
                      & Re   & \underline{\textbf{87.27}} & 86.81 & 71.90 & 87.26 & 77.45 & 86.51 & 71.90 & 83.58 & 71.84 \\
                      & F1   & \underline{\textbf{85.40}} & 85.00 & 67.80 & 80.74 & 77.21 & 84.40 & 67.81 & 82.54 & 79.62 \\ \hline
\end{tabular}
}
\end{table*}

\comment{
\begin{table*}[!h]
    \centering
    \caption{Performance comparison of \textsc{FedKO} and DÏoT with baseline models across datasets. Metrics with the best and second-best performance are \textbf{bold} and \underline{underline}, respectively.}
    \label{tab:DIoT}
    
    \scalebox{0.9}{
    \begin{tabular}{|c|c||c||c|c|c|c|c|}
        
        \hline
        \multirow{2}{*}{\textbf{Dataset}} & \multirow{2}{*}{\textbf{Metric}} & \multirow{2}{*}{\textbf{\textsc{FedKO}}} & \multicolumn{4}{c|}{\textbf{DÏoT}} 
        \\
        \cline{4-7}
        &  & 
        & \textbf{LSTM-AE} & \textbf{USAD} & \textbf{GDN}& \textbf{TranAD} % & \textbf{PUAD}
        \\
        \hline
        \hline
        \multirow{5}{*}{\textbf{SMD}}
        & AUC & 68.60 & 69.61 & \textbf{70.49} & 68.48 & 62.76 %&  \underline{69.53} 
        \\
        & Pre & \underline{76.25} & 56.79 & 54.05 & 73.53 & 41.53 %& \textbf{79.26} 
        \\
        & Recall & \textbf{79.75} & 53.90 & 71.05 & 63.48 & 41.17 %& \underline{69.85} 
        \\
        & F1 & \textbf{77.95}  & 55.31 & 61.39 & 68.13 & 41.36 %& \underline{74.26} 
        \\
        \hline
        \multirow{5}{*}{\textbf{MSL}}
        & AUC & 56.74 & \underline{58.98} & 56.25 & 56.49 & 58.39  %& \textbf{60.31}  
        \\
        & Pre & \underline{83.61}  & 53.86 & 64.57 & 73.27 & 61.06  %& \textbf{86.38}
        \\ 
        & Recall & \textbf{87.27}  & 72.05 & 72.46 & 86.21  & 86.87  %& \underline{72.25} 
        \\
        & F1 & \textbf{85.40} & 61.64 & 68.28 & 79.21 & 74.90  %& \underline{78.69} 
        \\
        \hline
    \end{tabular}}
\end{table*}
}

We extend our comparative analysis by including different federated learning (FL) methods (Scaffold~\cite{scaffold}, FedProx~\cite{fedprox}, and DÏoT~\cite{diot}) alongside \textsc{FedKO} to affirm its efficacy. The comparative table demonstrates \textsc{FedKO}'s consistently superior and balanced performance across various metrics and datasets against baseline models, as shown in Table~\ref{tab:performance_fl}. %and ~\ref{tab:DIoT}.

\subsection{Ablation and Parameter Sensitivity Study}
\label{ap:ablation}

\begin{table}[t]
\centering
\caption{Impact of FedKO's components.}
\label{tab:ablation}
\scalebox{0.9}{
\begin{tabular}{lccc}
\hline
\textbf{Variant}      & \textbf{Precision} & \textbf{Recall} & \textbf{F1-Score} \\ \hline
\textsc{FedKO}               & 97.55                   & 89.89                & 93.56                  \\
w/o Outer           & 90.09                   & 89.11                & 89.59                  \\
w/o Inner           & 92.97                   & 89.03                & 90.95                  \\
w/o SpecReg         & 96.38                   & 89.11                & 92.60                  \\  \hline
\end{tabular}}
\end{table}

\begin{table}[t]
\centering
\caption{Impact of $\beta$ values on performance.}
\label{tab:beta}
\scalebox{0.9}{
\begin{tabular}{c|cccccc}
\hline
\textbf{$\beta$} & \textbf{0} & \textbf{0.1} & \textbf{0.3} & \textbf{0.5} & \textbf{0.7} & \textbf{0.9} \\ \hline
\textbf{Pre} & 96.38 & 96.44 & 97.07 & 98.22 & 96.65 & 95.55 \\
\textbf{Re}    & 85.63 & 90.10 & 90.10 & 90.10 & 90.10 & 90.10 \\
\textbf{F1} & 90.68 & 93.16 & 93.45 & 93.98 & 93.25 & 92.75 \\ \hline
\end{tabular}}
\end{table}

\begin{table}[!t]
\centering
\caption{Impact of device rates on performance.}
\label{tab:client_rate}
\scalebox{0.9}{
\begin{tabular}{c|cccc}
\hline
\textbf{Device Rates} & \textbf{10\%} & \textbf{25\%} & \textbf{50\%} & \textbf{100\%} \\ \hline
\textbf{Pre} & 96.71 & 98.22 & 97.07 & 99.22 \\
\textbf{Re}    & 85.63 & 90.10 & 90.11 & 89.73 \\
\textbf{F1}  & 90.83 & 93.98 & 93.16 & 94.37 \\ \hline
\end{tabular}}
\vspace{-10pt}
\end{table}

\subsubsection{Effects of \textsc{FedKO}'s components} 
%We use PSM dataset to train \textsc{FedKO} and its variants: (1) without (w/o) outer level; (2) w/o inner level; (3) w/o spectral regularization (w/o SpecReg); (4) non-weighted aggregation ($\beta$ = 0). As shown in Fig~\ref{fig:ablation}, FedKO only achieves the best performance when integrating all framework components.
We evaluate the individual contributions of key components in \textsc{FedKO} on PSM, including its four variants: (1) without (w/o) outer level; (2) w/o inner level; and (3) w/o spectral regularization (w/o SpecReg). The study, detailed in Table~\ref{tab:ablation}, showcases that the optimal performance of \textsc{FedKO} necessitates the integration of all framework components. Removing the outer level, responsible for global updates, or the inner level, which manages local computations, significantly impairs the model's effectiveness. Similarly, omitting spectral regularization diminish performance, underscoring their roles in enhancing generalizability and adapting to node-specific data variations.

\subsubsection{Effects of $\beta$ and client rates} We explore the impact of varying $\beta$ values on \textsc{FedKO}'s performance with the PSM dataset. As shown in Table~\ref{tab:beta}, moderate $\beta$ values (0.5-0.7) enhance robustness by reducing noise and preserving history. Larger values (e.g., 0.9) may hinder adaptation to new updates and perpetuate past biases, while lower values (e.g., 0.1) only favors recent updates, compromising client data variability. Regarding the participation rate, the results in Table~\ref{tab:client_rate} highlight that an appropriated sub-client rate (e.g., 25\%) can achieve on-par performance with that of full clients. This suggests that engaging a smaller subset of clients is both practical and effective in maintaining high model performance while significantly reducing resource usage and network load.
%moderate $\beta$ values (0.5-0.7) strike an optimal balance, enhancing model robustness by reducing noise and effectively preserving historical data. Higher $\beta$ values (e.g., 0.9) tend to prioritize outdated information, resulting in reduced adaptability and perpetuating past biases. Conversely, lower $\beta$ values (e.g., 0.1) focus excessively on recent updates, neglecting valuable historical context.

\subsubsection{Effects of the Dimension of Koopman Operator and the Size of Reservoir Layer}

\begin{figure}[t]
    \vspace{-5pt}
	\centering
 	\begin{subfigure}{.47\linewidth}
		\centering
		\includegraphics[width=\textwidth]{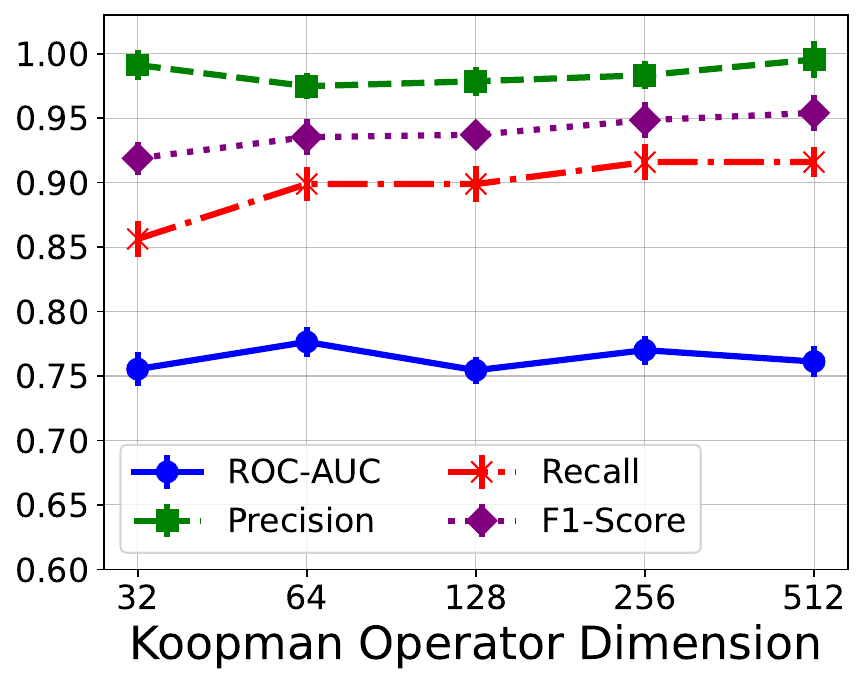}
        \vspace{-15pt}
		\caption{PSM}
		\label{fig:unsw}
	\end{subfigure}%
	\begin{subfigure}{.47\linewidth}
		\centering
		\includegraphics[width=\textwidth]{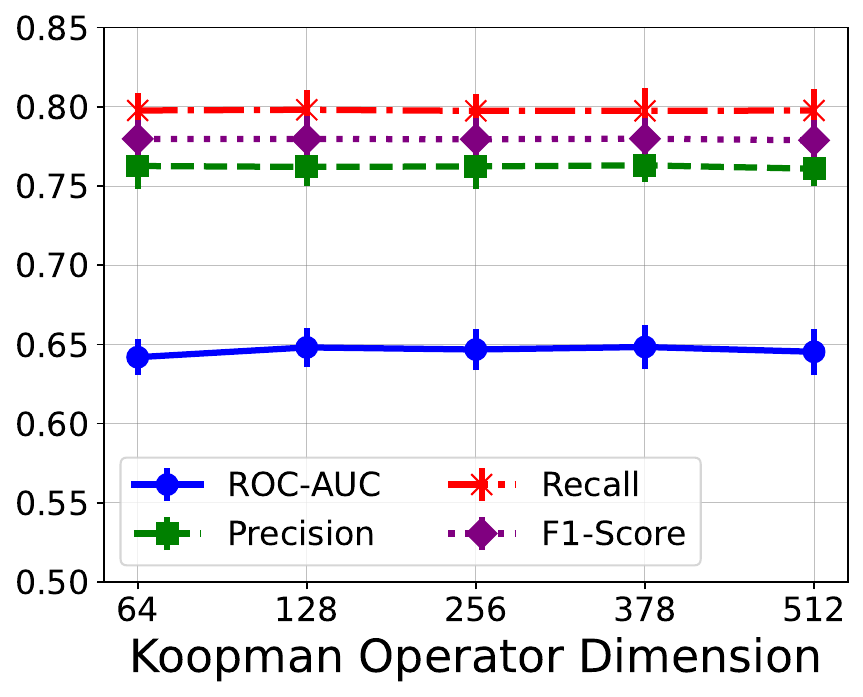}
        \vspace{-15pt}
		\caption{SMD}
		\label{fig:ton}
	\end{subfigure}
	%\label{fig:repochs}
	\caption{\textsc{FedKO} with various Koopman Operator dimensions.}
    \label{fig:koopman_size}
	%\vspace{-10pt}
\end{figure}

\begin{figure}[t]
    \vspace{-5pt}
	\centering
 	\begin{subfigure}{.47\linewidth}
		\centering
		\includegraphics[width=\textwidth]{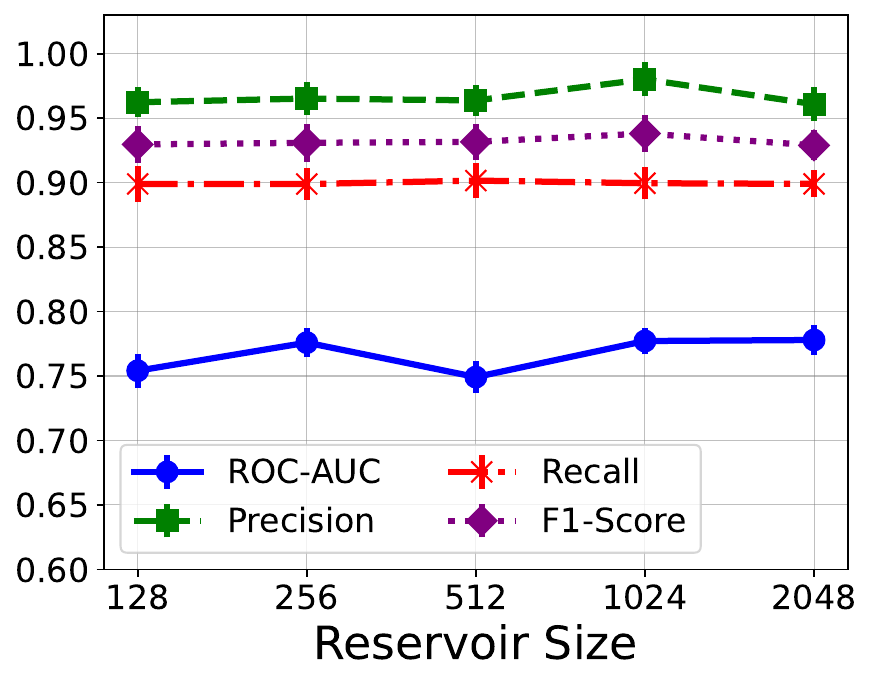}
        %\vspace{-15pt}
		\caption{PSM}
		\label{fig:unsw}
	\end{subfigure}%
	\begin{subfigure}{.47\linewidth}
		\centering
		\includegraphics[width=\textwidth]{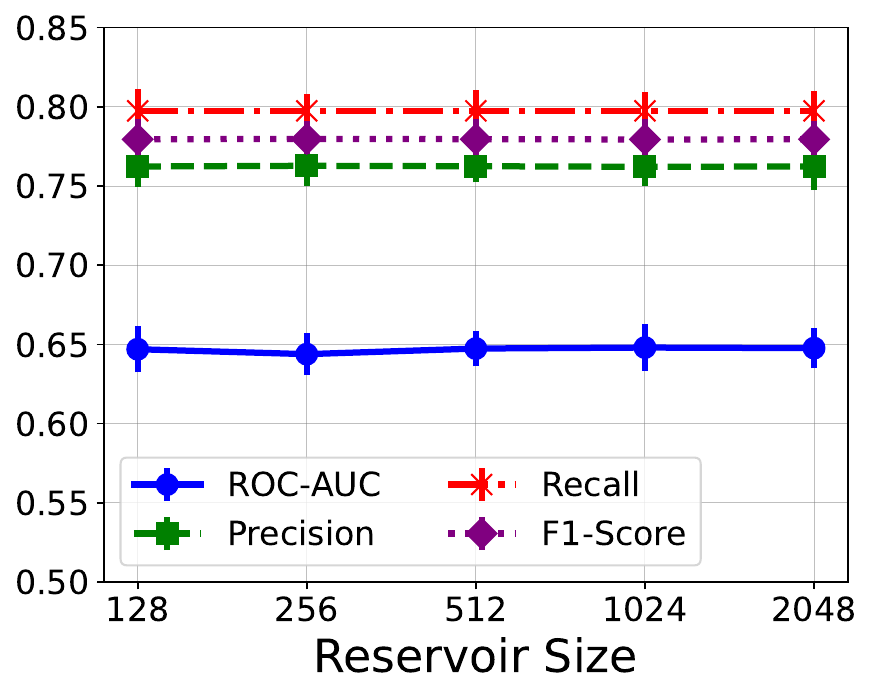}
        %\vspace{-15pt}
		\caption{SMD}
		\label{fig:ton}
	\end{subfigure}
	%\label{fig:repochs}
	\caption{\textsc{FedKO} with different sizes of reservoir layers.}
    \label{fig:reservoir_size}
	\vspace{-10pt}
\end{figure}

Evaluating \textsc{FedKO} across different dimensions of the Koopman Operator with the PSM and SMD datasets reveals consistent performance metrics, as shown in~\ref{fig:koopman_size}. Despite varying operator sizes, \textsc{FedKO} demonstrates stable effectiveness in MTAD across both datasets, indicating minimal impact of the Koopman Operator's dimension on the model's performance. This highlights \textsc{FedKO}'s reliability and adaptability to different operator sizes, thus establishing \textsc{FedKO} as a flexible solution for different IoT contexts.

%In the evaluation of \textsc{FedKO}'s performance across diverse dimensions of the Koopman Operator, utilizing the PSM and SMD datasets, we discovered a remarkable uniformity in performance indicators regardless of operator size. As illustrated in~\Cref{fig:koopman_size}, the results consistently affirm the resilience of \textsc{FedKO} against variations in the Koopman Operator's dimension. This observation was consistent across both datasets, where the key metrics exhibited minimal variation, underscoring the model's stable proficiency in accurately identifying and categorizing instances, independent of the operator's dimension. Such uniform performance not only underscores the dependability of \textsc{FedKO} but also its versatility in adapting to a range of operator sizes. This adaptability reinforces its potential for broad application in scenarios where the dimension of the Koopman Operator may differ, making \textsc{FedKO} a versatile tool in various analytical contexts.

%\subsubsection{Effects of }

The comparison of \textsc{FedKO} using different reservoir sizes with the PSM and SMD datasets also reveals uniform performance metrics, as depicted in Fig.~\ref{fig:reservoir_size}. ROC-AUC values across reservoir sizes consistently demonstrate the model's effective class differentiation. Precision remains high for all sizes, while Recall and F1-Scores show little variation with reservoir size changes. This consistent performance across varying reservoir dimensions highlights \textsc{FedKO}'s robustness, affirming that its effectiveness and reliability are largely unaffected by the reservoir layer's size.
